# Supplementary material for: Overwatch: Learning Patterns in Code Edit Sequences
Source: arXiv:2207.12456 source file (2022-07-25)
Supplement: Supplementary file 1 [file appendix.tex]

\section{APPENDIX}

\subsection{Algorithm for Anti-Unification}
% New definitions
\algnewcommand\algorithmicswitch{\textbf{switch}}
\algnewcommand\algorithmiccase{\textbf{case}}
\algnewcommand\algorithmicassert{\texttt{assert}}
\algnewcommand\algorithmicdefault{\textbf{default}}
\algnewcommand\Assert[1]{\State \algorithmicassert(#1)}%
% New "environments"
\algdef{SE}[SWITCH]{Switch}{EndSwitch}[1]{\algorithmicswitch\ #1\ \algorithmicdo}{\algorithmicend\ \algorithmicswitch}%
\algdef{SE}[CASE]{Case}{EndCase}[1]{\algorithmiccase\ #1}{\algorithmicend\ \algorithmiccase}%
\algdef{SE}[DEFAULT]{Default}{EndDefault}[0]{\algorithmicdefault}{\algorithmicend\ \algorithmicdefault}%
\algtext*{EndSwitch}%
\algtext*{EndCase}%
\algtext*{EndDefault}%

\begin{algorithm}
  \small
  \begin{algorithmic}[1]
    \Require Two edit sequence patterns $\langle \tpltseq_1=\etplt_1^1\ldots,\etplt_n^1, \tmprel_1 \rangle, \langle \tpltseq_2=\etplt_1^2\ldots,\etplt_n^2, \tmprel_2 \rangle$
    \Ensure A new edit sequence pattern $\langle \tpltseq, \tmprel \rangle$ merged from two given patterns, the cost $C$.
    \Function{AntiUnify}{$
        \langle \tpltseq_1=\etplt_1^1\ldots,\etplt_n^1, \tmprel_1 \rangle,
        \langle \tpltseq_2=\etplt_1^2\ldots,\etplt_n^2, \tmprel_2 \rangle
    $}
      \State $\tmprel,\substitution_1,\substitution_2,\mathsf{CurEqRel}
        \gets \emptyset, \emptyset, \emptyset, \emptyset$
      \For{$i \in \{ 1, \ldots, n\}$}
        \State $\substitution_1', \substitution_2', C', \tplt_{i,\pre} \gets $ \Call{AntiUnifyTemplate}{$\tplt_{i,\pre}^1$, $\tplt_{i,\pre}^2$, $\mathsf{CurEqRel}$}
        \State $
            C, \substitution_1, \substitution_2, \mathsf{CurEqRel} \gets
            C + C',
            \substitution_1 \cup \substitution_1',
            \substitution_2 \cup \substitution_2',
            \mathsf{CurEqRel} \cup \{(\substitution_1(\hole), \substitution_2(\hole))
            \mid \hole \in \tplt_{i,\pre}\}$
        
         \State $\substitution_1', \substitution_2', C', \tplt_{i,\post} \gets $ \Call{AntiUnifyTemplate}{$\tplt_{i,\post}^1$, $\tplt_{i,\post}^2$, $\mathsf{CurEqRel}$}
        \State $C \gets C + C', \substitution_1 \gets \substitution_1 \cup \substitution_1', \substitution_2 \gets \substitution_2 \cup \substitution_2', \mathsf{CurEqRel} \gets \mathsf{CurEqRel} \cup \{(\substitution_1(\hole), \substitution_2(\hole))|\hole \in \tplt_{i,\post}\}$
        \State Add $\tplt_{i,\pre} \to \tplt_{i,\post}$ to $\tpltseq$
      \EndFor
      \State Add relations to $\tmprel$ based on $\substitution_1, \substitution_2, \tmprel_1, \tmprel_2$
      \State $C \gets \frac{C}{|\tpltseq_1| + |\tpltseq_2|}$
      \State \Return $\langle \tpltseq, \tmprel \rangle, C$
      \EndFunction
    \Function{AntiUnifyChildren}{$c_1^1,\dots,c_p^1$, $c_1^2,\dots,c_q^2$, $\mathsf{CurEqRel}$} 
    % \Comment{Find a template  and $\substitution_1, \substitution_2$ such that 1) $\substitution_1(c_1,\dots,c_r) = c_1^1,\dots,c_p^1, \substitution_2(c_1,\dots,c_r) = c_1^2,\dots,c_q^2$, and 2) the cost $C'=\sum_{\hole \in \tplt \wedge (\substitution_1(H), \substitution_2(H)\notin \mathsf{CurEqRel}} \cost(\hole)$ is minimized.}
        \For{$1 \le i \le p$, $1 \le j \le q$} \Comment{Dynamic programming}
            \If{$c_i^1$ is already a hole}
                \State $C_1 \gets f_{i-1,j}+0.5$ if $(c_i^1, \epsilon) \not \in \mathsf{CurEqRel}$, otherwise, $C_1 \gets 0$
            \Else
                 \State $C_1 \gets f_{i-1,j}+|c_i^1|+0.5$ if $(c_i^1, \epsilon) \not \in \mathsf{CurEqRel}$, otherwise, $C_1 \gets 0$
            \EndIf
            \If{$c_j^2$ is already a hole}
                \State $C_2 \gets f_{i,j-1}+0.5$ if $(\epsilon, c_j^2) \not \in \mathsf{CurEqRel}$, otherwise, $C_2 \gets 0$
            \Else
                \State $C_2 \gets f_{i,j-1}+|c_j^2|+0.5$ if $(\epsilon, c_j^2) \not \in \mathsf{CurEqRel}$, otherwise, $C_2 \gets 0$
            \EndIf
            \State $C_3 \gets f_{i-1,j-1}+$\Call{AntiUnifyTemplate}{$c_i^1$, $c_j^2$, $\mathsf{CurEqRel}$}\code{.cost}$)$
            \Switch{$C_1, C_2, C_3$}
                \Case{$C_1 \le C_2 \wedge C_1 \le C_3$}
                    \State $f_{i,j} \gets C_1$ \Comment{Create a hole $\hole$ such that $\substitution_1(\hole)=c_i^1, \substitution_2(\hole)=\epsilon$}
                \EndCase
                \Case{$C_2 \le C_1 \wedge C_2 \le C_3$}
                    \State $f_{i,j} \gets C_2$ \Comment{Create a hole $\hole$ such that $\substitution_1(\hole)=\epsilon, \substitution_2(\hole)=c_j^2$}
                \EndCase
                \Default 
                    \State $f_{i,j} \gets C_3$ \Comment{Get template $\tplt'$ from AntiUnifyTemplate such that $\substitution_1(\tplt')=c_i^1, \substitution_2(\tplt')=c_j^2$}
                \EndDefault
            \EndSwitch
        \EndFor
        \State $C' \gets f_{p,q}$
        \State Get $\tplt, \substitution_1, \substitution_2$ from the optimal trace of dynamic programming.
        \State \Return $\substitution_1, \substitution_2, C', \tplt$
    \EndFunction
    
    \Function{AntiUnifyTemplate}{$T_1$, $T_2$, $\mathsf{CurEqRel}$} \Comment{Returns two substitutions, the cost, and the anti-unified edit template.}
        \Switch{$T_1, T_2$}
            \Case{At least one of $T_1, T_2$ is a hole or \code{$T_1$.root $\neq$ $T_2$.root}}
                \State $\substitution_1 \gets \{\hole \mapsto T_1\}, \substitution_2 \gets \{\hole \mapsto T_2\}$
                \State $C' \gets \cost(\hole, \substitution_1, \substitution_2)$ if $(T_1, T_2) \notin \mathsf{CurEqRel}$, otherwise, $C' \gets 0$ 
                \State \Return $\substitution_1, \substitution_2, C', \hole$ 
            \EndCase
            \Case{$T_1 = T_2$}
                \State \Return $\varnothing, \varnothing, 0, T_1$
            \EndCase
            \Default \Comment{\code{$T_1$.root = $T_2$.root}}
                \State \Return \Call{AntiUnifyChildren}{$T_1$\code{.children}, $T_2$\code{.children}, $\mathsf{CurEqRel}$} 
            \EndDefault
        \EndSwitch
    \EndFunction
  \end{algorithmic}
  \caption{The procedure of anti-unification and cost computation}
  \label{algo:anti-unification}
\end{algorithm}

Algorithm~\ref{algo:anti-unification} depicts the procedure for anti-unifying
two ESPs
$\langle \tpltseq = \etplt_1\ldots\etplt_n, \tmprel \rangle$ and 
$\langle \tpltseq' = \etplt_1'\ldots\etplt_n', \tmprel' \rangle$.
The algorithm returns
$\langle \tpltseq^* = \etplt_1^*\ldots\etplt_n^*, \tmprel^* \rangle$
The algorithm maintains two substitutions $\substitution$ and $\substitution'$.
At the end of the procedure, we will have that
$\substitution(\etplt_i^*) = \etplt_i$ and
$\substitution'(\etplt_i^*) = \etplt_i'$.

Formally, The cost of merging two ESPs $\langle \tpltseq,
\tmprel \rangle$ and $\langle \tpltseq', \tmprel' \rangle$ to obtain a new ESP $\langle \tpltseq^*, \tmprel^* \rangle$ and two substitutions $\substitution$ and $\substitution'$, where $\substitution(\tpltseq^*) = \tpltseq$ and $\substitution'(\tpltseq^*) = \tpltseq'$, is defined as follows:
\begin{align}
    &\cost(\tpltseq^*, \tmprel^*, \substitution, \substitution') =
      \frac
      {
        |\tpltseq^*|
        - |\mathsf{Holes}(\tpltseq^{*})|
        + \sum_{[\hole] \in \mathsf{Holes}(\tpltseq^{*})
            / \dependency_\mathsf{Eq}}
        \cost(\hole, \substitution, \substitution')
      }
      % {|\tpltseq^{\leftts}| + \tpltseq^{\rightts}|}\\
      {|\tpltseq| + |\tpltseq'|},\label{eq:mergecost}
    \\
    &\cost(\hole, \substitution, \substitution') = |\substitution(\hole)| + |\substitution'(\hole)| + \begin{cases}
\infty, & \text{both } \substitution(\hole)\ \substitution'(\hole) \text{ are }\epsilon\\
0, & \text{one of } \substitution(\hole)\ \substitution'(\hole) \text{ is hole and the other is }\epsilon\\
0.5, & \text{only one of } \substitution(\hole)\ \substitution'(\hole) \text{ is }\epsilon\\
-1.5, & \text{both } \substitution(\hole)\ \substitution'(\hole) \text{ are holes}\\
-0.5, & \text{otherwise}
\end{cases},\label{eq:holecost}
\end{align}
where $\mathsf{Holes}(\tpltseq^{*}) / \dependency_\mathsf{Eq}$ is the equivalence set of holes in $\tpltseq^*$ over the equivalence relation in temporal dependency $\tmprel^*$.
In Eq~\ref{eq:mergecost}, we penalize the cost of holes from different quotient sets because fewer quotient sets mean more equivalence relations discovered in the temporal dependency. 
In~\citet{revisar}
% \gustavo{I think this reference is wrong. I think you meant the Revisar work, not the Refazer work, which does not use anti-unification, right?} \yh{yes, I updated the reference}
, the hole cost is defined as $\cost(\hole, \substitution, \substitution') = |\substitution(\hole)| + |\substitution'(\hole)| - 1$.
We define the hole cost similarly in Eq~\ref{eq:holecost} but penalize or reward the cost according to different situations. 
Concretely, we forbid $\hole$ to be substituted as $\epsilon$ in both substitutions (case 1) and penalize $\epsilon$ (cases 2 and 3) to avoid generating too many holes that are substituted by $\epsilon$.
We reward the cost if there are already corresponding holes in two ESPs (case 4).

\subsection{Complete List of Edit Sequence Patterns}
\newcounter{counter}
\setcounter{counter}{1}
% \begin{longtable}[htbp]
% \centering

% \begin{landscape}\vspace{-4ex}
\begin{ThreePartTable}
\centering
\fontsize{7pt}{8pt}\selectfont
\begin{longtable}{llll}
\caption{Complete List of Edit Sequence Patterns learned by \technique}\\
\textbf{Category}              & \textbf{Id}            & \textbf{Pattern Description} & \textbf{Related Feature}\\
\toprule
\multirow{27}{*}{\makecell[l]{Workflow}}
                                      & \thecounter\stepcounter{counter} & Rename method decl $\rightarrow$ Rename method calls  & \textit{Rename Method} \\
                                      & \thecounter\stepcounter{counter}  & Insert variable decl $\rightarrow$ Replace constants with new variable & \textit{Introduce Local Variable} \\
                                      & \thecounter\stepcounter{counter}  & Insert parameter $\rightarrow$ Insert argument to callsites  & \textit{Insert parameter} \\
                                      & \thecounter\stepcounter{counter}  & Delete parameter $\rightarrow$ Delete argument from callsites & \textit{Delete parameter} \\
                                      & \thecounter\stepcounter{counter}  & Replace variable declaration by assignment $\rightarrow$ Insert new field  &\textit{Promote local variable to field}\\
                                       & \thecounter\stepcounter{counter}  & Insert Property $\rightarrow$ Insert Parameter $\rightarrow$ Insert Assignment &\textit{Initialize property} \\
                                       & \thecounter\stepcounter{counter}  & Delete arguments from method \emph{call}s $\rightarrow$ Delete Parameter from method declaration&\textit{Delete Parameter} \\
                                     & \thecounter\stepcounter{counter}  & Insert expression $\rightarrow$ Replace it by assignment & \textit{Introduce variable} \\
                                     & \thecounter\stepcounter{counter}  & Insert parameter in constructor, add assignment to the corresponding property &
                                     Insert Assignment\\
                                     & \thecounter\stepcounter{counter}  & Insert new assignment statement -> add \textit{var} to the LHS of the assignment &
                                     Introduce local\\
                                     %\priyanshu{Not sure}\\
                                     & \thecounter\stepcounter{counter}  & Insert new parameter to constructor -> Insert new property &
                                     Create property \\
                                     % \priyanshu{Not sure}\\
                                     & \thecounter\stepcounter{counter} & Change type in variable decl $\rightarrow$ Change constructor name in initializer &\textit{New Feature}\\
                                     & \thecounter\stepcounter{counter}  & Delete parameter $\rightarrow$ Delete assignment $\rightarrow$ Delete property &\textit{New Feature} \\
                                     & \thecounter\stepcounter{counter}  & Insert parameter with default value $\rightarrow$ Replace constants with parameter  &\textit{New Feature}\\
                                     & \thecounter\stepcounter{counter}  & Delete field $\rightarrow$ Delete assignment  &\textit{New Feature}\\
                                     & \thecounter\stepcounter{counter}  & Insert argument to callsite $\rightarrow$ Remove default parameter value  &\textit{New Feature}\\
                                     & \thecounter\stepcounter{counter}  & Insert variable declaration $\rightarrow$ Insert new variable as argument &\textit{New Feature}\\
                                     &\thecounter\stepcounter{counter}  & Insert return statement $\rightarrow$ Delete throw "NotImplementedException"  &\textit{New Feature}\\
                                     & \thecounter\stepcounter{counter}  & Add abstract to class decl $\rightarrow$ Add abstract to method decl  &\textit{New Feature}\\
                                     & \thecounter\stepcounter{counter}  & Add \textit{foreach} \{ \} $\rightarrow$ Wrap next statement within this block  &\textit{New Feature}\\
                                     & \thecounter\stepcounter{counter}  & Insert return statement $\rightarrow$ Delete throw "NotImplementedException"  &\textit{New Feature}\\
                                     & \thecounter\stepcounter{counter}  & Insert \textit{if \{\}} $\rightarrow$ Wrap next statement in the \emph{if} block&\textit{New Feature}\\
                                     & \thecounter\stepcounter{counter}  & Cut a statement $\rightarrow$ Paste the statement in an empty block  &\textit{New Feature}\\
                                     & \thecounter\stepcounter{counter}  & Declare a variable $\rightarrow$ Replace occurence of \textit{null} with the variable&\textit{New Feature}\\
                                     & \thecounter\stepcounter{counter}  & Delete a variable $\rightarrow$ Delete any expresion where the variable was used&\textit{New Feature}\\
                                     & \thecounter\stepcounter{counter}  & Delete a property$\rightarrow$ Delete any expresion where the property was used&\textit{New Feature}\\
                                     & \thecounter\stepcounter{counter}  & Insert a variable in an argument list$\rightarrow$ Delete expressions wherever variable used used&\textit{New Feature}\\
                                     
\midrule
\midrule
\multirow{24}{*}{\makecell[l]{Repeat}}  
                                    & \thecounter\stepcounter{counter}  & Remove `this' in multiple locations & \textit{Remove unnecessary qualifier ``this''} \\ 
                                    & \thecounter\stepcounter{counter}  & Remove `cast' in multiple locations & \textit{Remove unnecessary cast}\\
                                    & \thecounter\stepcounter{counter}  & Add prefix `\_' to name & \textit{Fix naming convention} \\
                                    & \thecounter\stepcounter{counter}  & Replace constant with local variable &\textit{Introduce Local} \\
                                    & \thecounter\stepcounter{counter}  & Rename a variable in many locations &\textit{Rename Variable} \\
                                    & \thecounter\stepcounter{counter}  & Rename a property &\textit{Rename Propertyl} \\
                                    & \thecounter\stepcounter{counter}  & Converting static method calls to virtual in multiple locations  & \textit{New Feature} \\ 
                                    & \thecounter\stepcounter{counter}  & Remove a method invocation from many locations & \textit{New Feature}\\
                                    & \thecounter\stepcounter{counter}  & Replace an expression by a method invocation & \textit{New Feature} \\
                                    & \thecounter\stepcounter{counter}  & Change modifiers for multiple locations/properties  &\textit{New Feature}\\
                                     & \thecounter\stepcounter{counter}  & Change modifiers for multiple locations/properties  &\textit{New Feature}\\
                                     & \thecounter\stepcounter{counter}  & Replace a specific constant at multiple locations  &\textit{New Feature}\\
                                     & \thecounter\stepcounter{counter}  & Replace a specific data type multiple locations  &\textit{New Feature}\\
                                     & \thecounter\stepcounter{counter}  & Delete a specific method call for multiple objects  &\textit{New Feature}\\
                                     & \thecounter\stepcounter{counter}  & Delete a specific constant string at multiple locations  &\textit{New Feature}\\
                                     & \thecounter\stepcounter{counter}  & Replace object by its member at multiple locations  &\textit{New Feature}\\
                                     & \thecounter\stepcounter{counter}  & Replace reference to a \emph{member} by reference to an \emph{object} of the class  &\textit{New Feature}\\
                                     & \thecounter\stepcounter{counter}  & Delete a specific expression from multiple locations &\textit{New Feature}\\
                                     & \thecounter\stepcounter{counter}  & Delete a specific statement from multiple locations &\textit{New Feature}\\
                                     & \thecounter\stepcounter{counter}  & Change a specific generic type in multiple locations &\textit{New Feature}\\
                                     & \thecounter\stepcounter{counter}  & Change a specific method call in multiple locations &\textit{New Feature}\\
                                     & \thecounter\stepcounter{counter}  & Remove multiple properties of a class one after the other &\textit{New Feature}\\
                                     & \thecounter\stepcounter{counter}  & Replace method invocation by another method &\textit{New Feature}\\
                                     & \thecounter\stepcounter{counter}  & Delete an argument in a specific  method call at multiple locations &\textit{New Feature}\\

\bottomrule
\end{longtable}
% \begin{tablenotes}[para]
% \item[1] Applicable to fields \item[2] Applicable to variable declarations and assignments \item[3] Applicable to fields, properties and local variables
% \end{tablenotes}
\end{ThreePartTable}

\vspace{-2ex}
% \end{landscape}
% \end{longtable}
